# Supplementary material for: A CMOS-compatible Ising Machine with Bistable Nodes
Source: arXiv:2007.06665 source file (2022-12-02)
Supplement: Supplementary file 1 [file 6appendix.tex]

\begin{appendices}

\section{MATLAB code for Max-Cut problem.}
% \label{app:code}

% \begin{lstlisting}[caption={BRIM Sample Code (without annealing or spin-flip)}\label{app:code}]
% function sample

%     % Graph problem with maximum cut value of 18.2
%     src = [1  1  1 1  2.0  2 2.0 3  3.0 4  4  5.0];
%     dst = [2  3  5 6  3.0  4 6.0 4  5.0 5  6  6.0];
%     wgt = [1 -1 -2 6 -0.2 -2 4.4 4 -4.4 6 -1 -0.2];
%     spin= length(unique([src dst]));
%     W1  = sparse(src, dst, wgt, spin, spin));
%     W2  = sparse(dst, src, wgt, spin, spin));
%     W   = full(W1 + W2);

%     % Hardware Parameters
%     C   = 49e-15;               % Node capacitor
%     Rc  = 31e3;                 % Coupling resistors
%     ziv = @(v) (-2.1563e-05 .* v.^5) + ... % Diode
%               (  1.017e-04 .* v.^3) + ...  % ...
%               ( -2.231e-05 .* v);          % ...
               
%     % Graph to Ising transformation
%     J   = -W ./ Rc;

%     % Solve BRIM system
%     I   = rand(spin,1) - 0.5;   % Initial states
%     T   = [0 1e-9];             % Annealing time
%     sol = ode45(@(t,v)brim(v,J,C,ziv), T, I);

%     % Brim Model
%     function dvdt = brim(v, J, C, ziv)

%         % BRIM differential equation
%         dvdt = ((J * v) - ziv(v)) ./ C;

%         % Model diode operation range
%         dvdt((v < -1) & (dvdt < 0)) = 0;
%         dvdt((v >  1) & (dvdt > 0)) = 0;
%     end
% end
% \end{lstlisting}

% \section{New Best Solution(s) Found for Gset}
% In this section we list any new solutions found during our experimentation;
% % \bf{G29}: \seqsplit{3B1495ABF04C49B47791A2061593BC11AB9FEA62F8E67AC4FC95F0C7CE88519DA826E525D6D7B341F47929BBA451FDEDECA44A930665A725F70D9A487A42A6AC6DC975558B0CD30DFD533EDD9740B4E58AE4954490A59E08E6A21904F4A30FDE2E44F022F3CAEBC79F0A87E21CAD7B2E88F0FFE5A4B5AF90E9EC0D8D9357FD05ACB77D70B4CC06B1641CEAE6533ADE6FAE4CC3F3648B8F9C87A8EF1F2784BF1875136199380A256CB0E250122F122615E0A9FB23B6E3FC66A6BB33AB247569985CFC6CB27DD4F4B7FE2D374F68076F70456AF38C75C937D3C636105ED2732CBCE33725BE1EBDC453F37098A1C384D2630147625A286CCFF83BD8}

\end{appendices}
